# Supplementary material for: TAR3D: Creating High-Quality 3D Assets via Next-Part Prediction
Source: arXiv:2412.16919 source file (2025-08-09)
Supplement: Supplementary file 1 [file suppl_ito3d.tex]

% \clearpage
\begin{figure*}[htbp]
  \centering
  \footnotesize
  % \fbox{\rule{0pt}{4in} \rule{0.9\linewidth}{0pt}}
   \includegraphics[width=\linewidth]{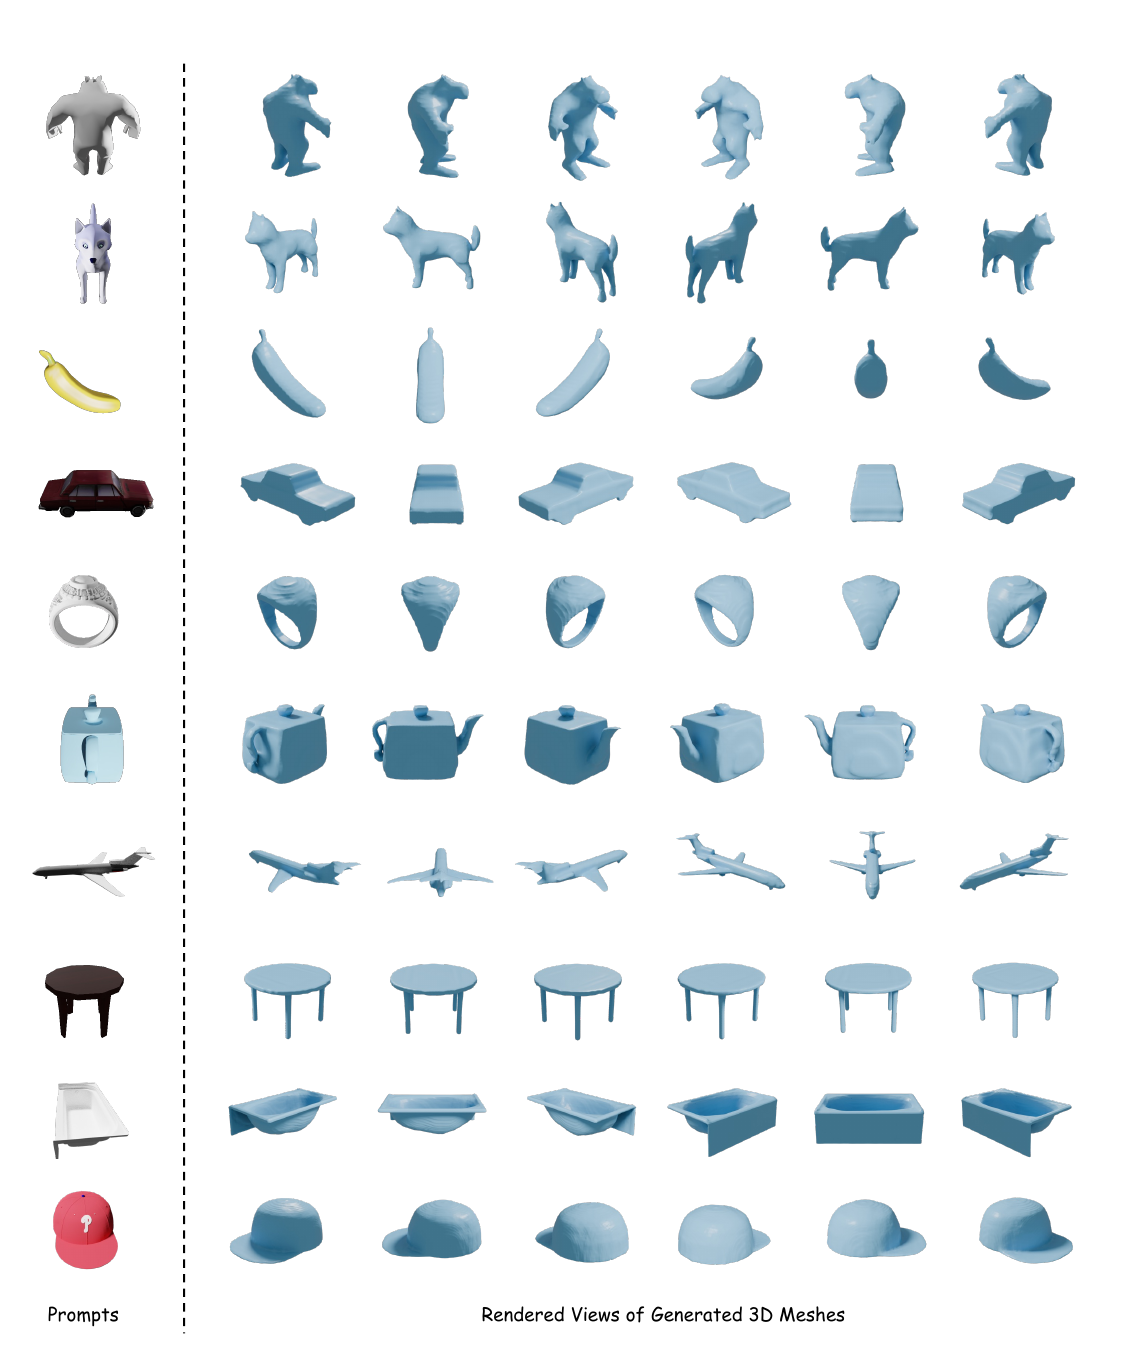}

   \caption{Given a wide range of input images from the benchmark datasets, \ie ShapeNet and Objaverse, our \ourMthd{} model is capable of inferring the full picture of the primary objects and producing high-quality 3D meshes that adhere to them.}
   \label{fig:suppl_ito3d}
\end{figure*}
% \clearpage
% \raggedbottom

% \renewcommand{\floatpagefraction}{1.0}
% \renewcommand{\textfraction}{0.0}

% \WarningFilter{latex}{Text page contains only floats} % 忽略特定警告
