# Supplementary material for: TAR3D: Creating High-Quality 3D Assets via Next-Part Prediction
Source: arXiv:2412.16919 source file (2025-08-09)
Supplement: Supplementary file 3 [file suppl_tto3d.tex]

\begin{figure*}[t]
  \centering
  \footnotesize
  % \fbox{\rule{0pt}{4in} \rule{0.9\linewidth}{0pt}}
   \includegraphics[width=.98\linewidth]{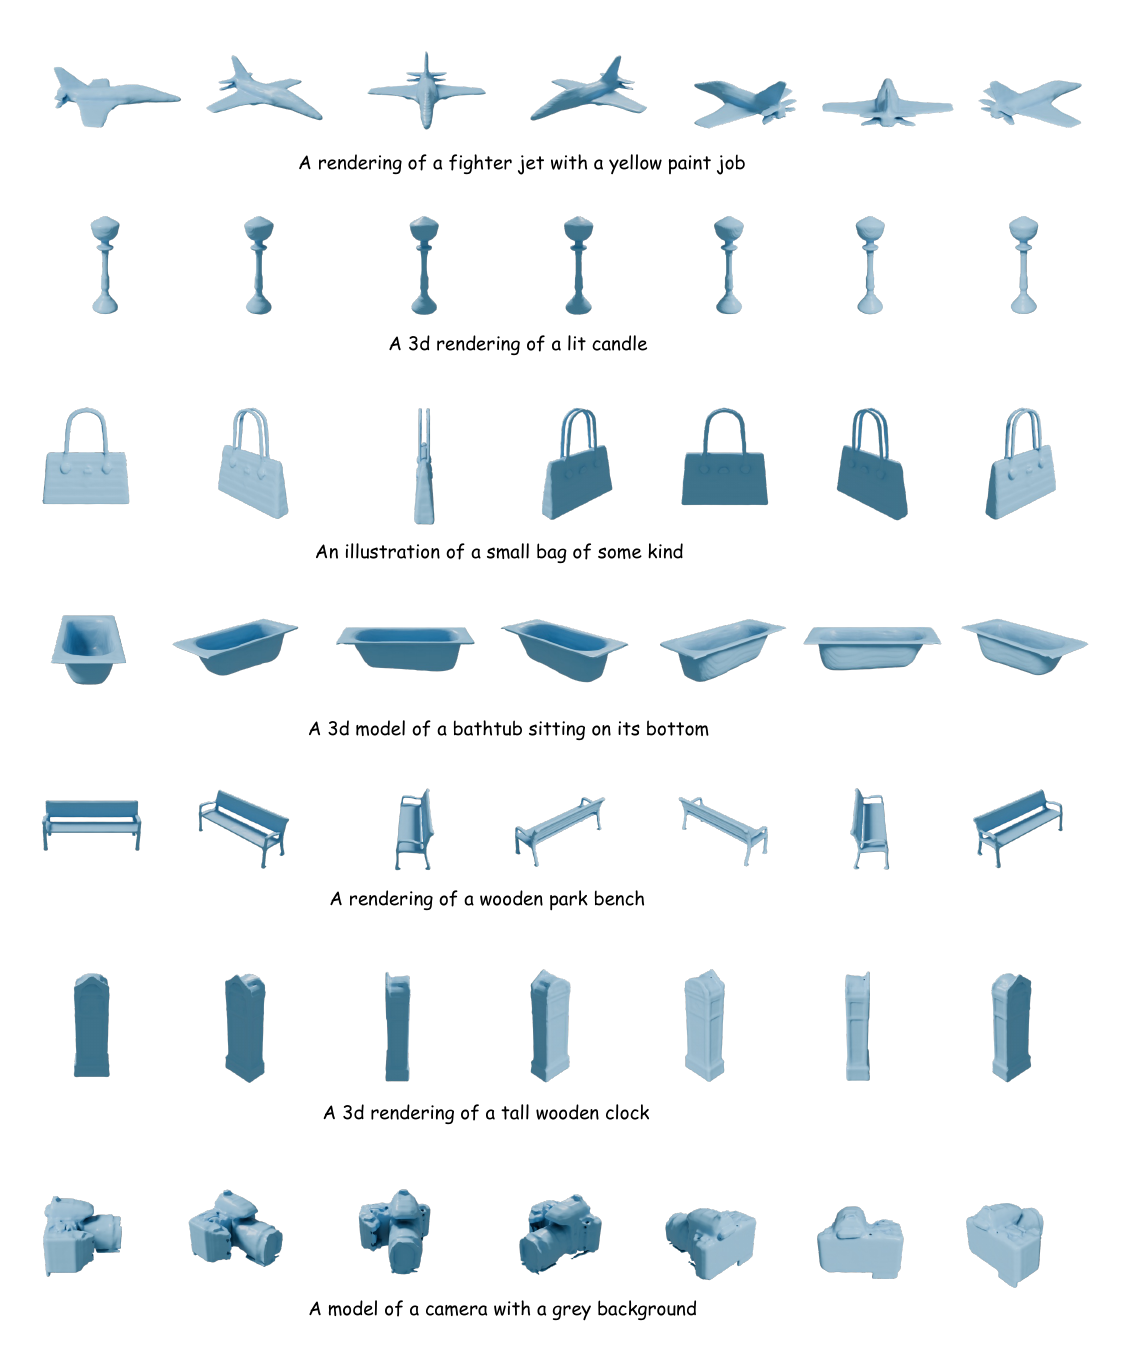}

   \caption{Qualitative results of our \ourMthd{} on a broad spectrum of text prompts.
   It can be observed that these 3D meshes created by our \ourMthd{} model are semantically faithful to the textual descriptions.
   }
   % \vspace{-5pt}
   \label{fig:suppl_tto3d}
\end{figure*}
